# Supplementary material for: Automatic Root Cause Analysis via Large Language Models for Cloud Incidents
Source: arXiv:2305.15778 source file (2023-11-13)
Supplement: Supplementary file 1 [file appendix.tex]

\begin{figure}[h]
\centering
\includegraphics[width=0.4 \textwidth]{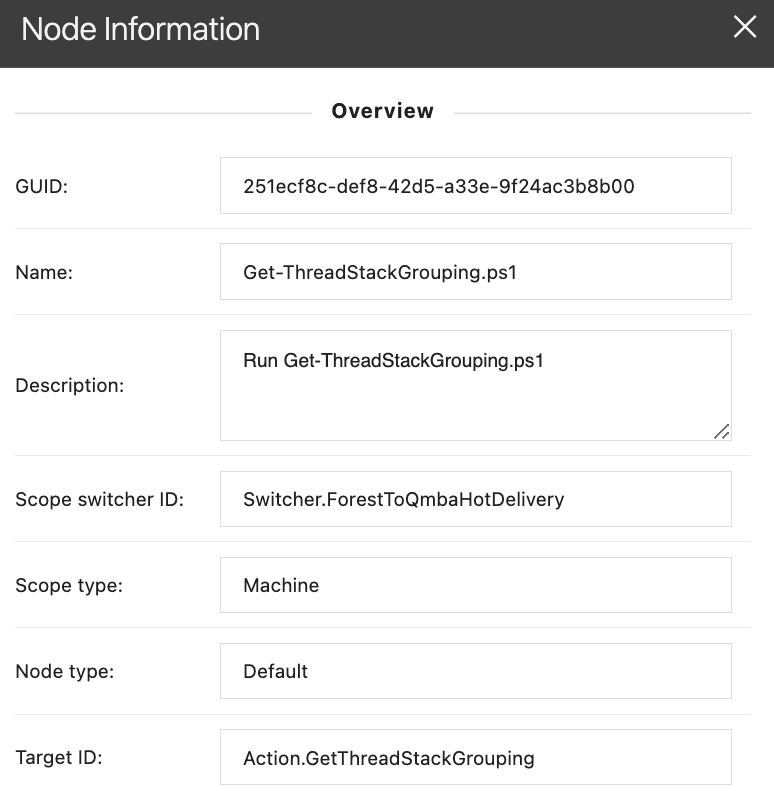}
\caption{
Web-based UI of \name{} for handler construction. 
}
\label{fig:gui}
\end{figure}
 
To facilitate the building of the \name{} incident handler, 
we have implemented \name{}'s handler construction as a web application,
as shown in Figure~\ref{fig:gui}.

We have successfully deployed \name{}'s diagnostic information collection module across 30 teams within CompanyX. From these, we've selected the top 10 teams that utilize the most \name{} incident handlers. Table~\ref{table:team_summary} provides details about the average execution time and the count of active handlers for these selected teams.
 
\begin{table}[htbp]
\centering
\begin{tabular}{lcc}
\toprule
\multirow{2}{*}{Team} & Avg. exec. & Enabled  \\
& time (seconds) & handler  \\ 
\midrule
Team 1 & 841 & 213 \\
Team 2 & 378 & 204 \\
Team 3 & 106 & 88 \\
Team 4 & 449 & 42 \\
Team 5 & 136 & 41 \\
Team 6 & 91 & 34 \\
Team 7 & 449 & 32 \\
Team 8 & 255 & 32 \\
Team 9 & 323 & 31 \\
Team 10 & 22 & 18 \\
 
\bottomrule
\end{tabular}
\caption{Teams using \name{} to automatically collect diagnostic information.}
\label{table:team_summary}
\end{table}
